# Supplementary material for: Dynamical renormalization of electron-phonon coupling in conventional superconductors
Source: arXiv:2212.08117 ancillary file (2023-02-16)
Supplement: Supplementary file 1 [file SuppInfo.pdf]

# Supplementary information:
# Dynamical renormalization of electron-phonon coupling in conventional superconductors

Nina Girotto[1] and Dino Novko[1,*]

[1] *Institute of Physics, 10000 Zagreb, Croatia*

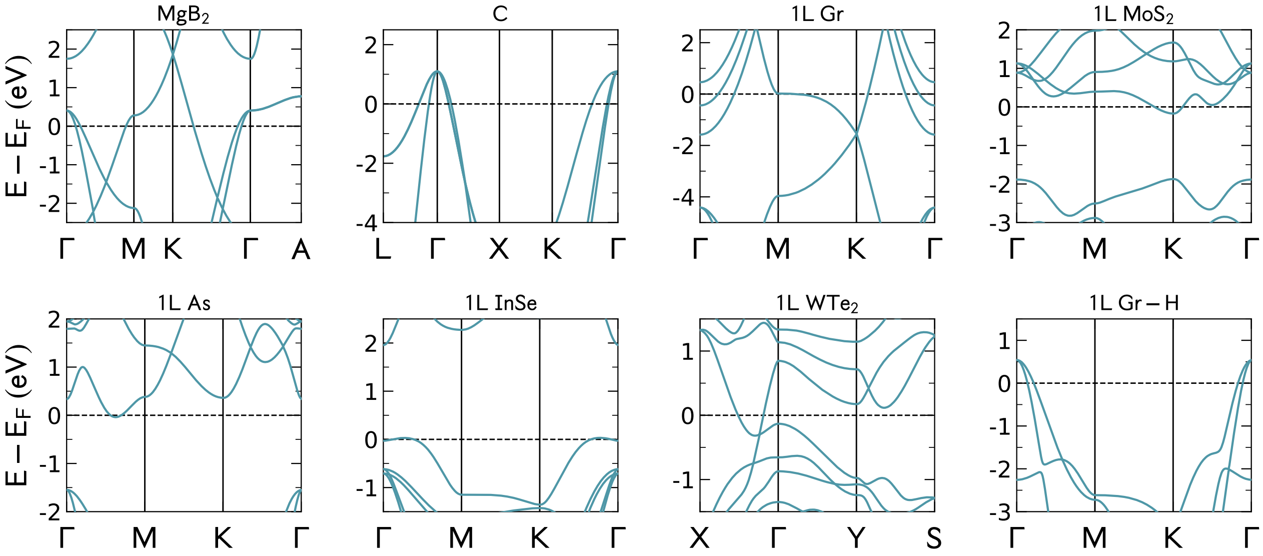


**Supplementary Figure 1**. Electronic band structures for various bulk and two-dimensional systems presented along the high-symmetry points of the first Brillouin zone. The results are shown for magnesium diboride ($MgB_2$), hole-doped diamond (C), highly electron-doped single-layer graphene (1L Gr), electron-doped single-layer molybdenum disulfide (1L $MoS_2$), electron-doped arsenene (1L As), hole-doped single-layer indium selenide (1L InSe), electron-doped single-layer wolfram ditelluride (1L $WTe_2$), and hole-doped graphane (1L Gr-H).

* dino.novko@gmail.com

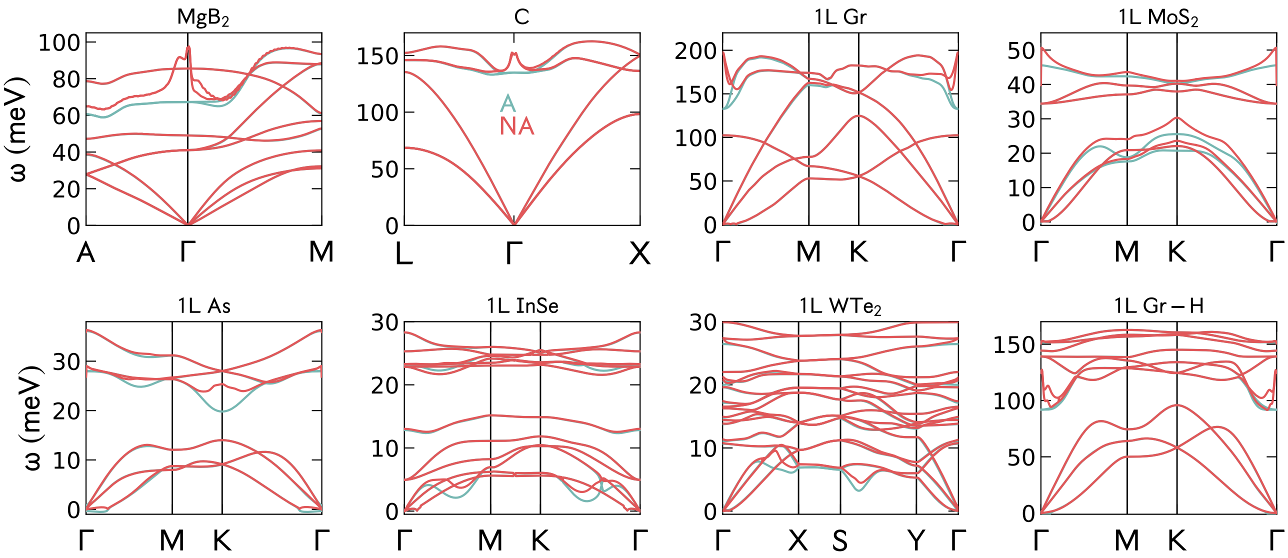


**Supplementary Figure 2**. Phonon dispersions along the high-symmetry points of the first Brillouin zone for various bulk and two-dimensional systems as obtained with standard adiabatic approach (as in DFPT [1]) and with the nonadiabatic corrections.

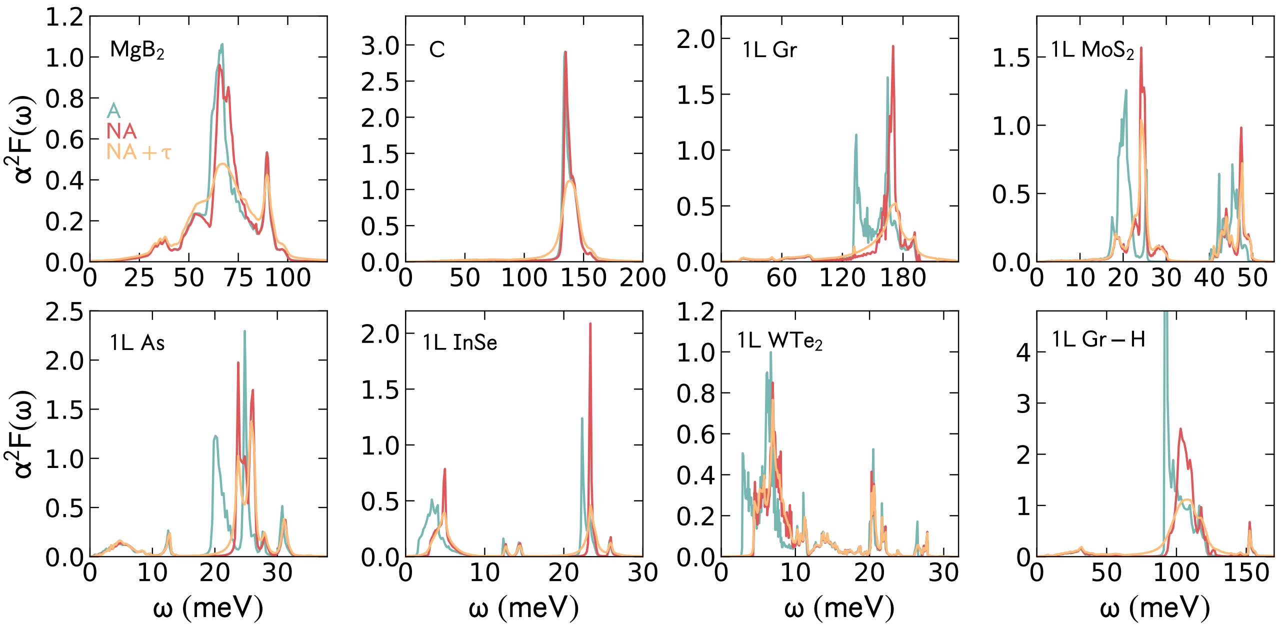


**Supplementary Figure 3**. Electron-phonon spectral (or Eliashberg) functions for various bulk and two-dimensional systems. The results are shown for three different approaches: adiabatic (A), where frequencies are obtained within the adiabatic DFPT and without momentum and branch-resolved phonon broadenings $\gamma_{\mathbf{q}\nu}$ (blue), nonadiabatic (NA), where frequencies are corrected with NA effects, while the corresponding NA phonon broadening due to EPC is not included (red), and full nonadiabatic (NA+$\tau$), where both NA frequency renormalization and NA phonon linewidth effects are taken into account (yellow).

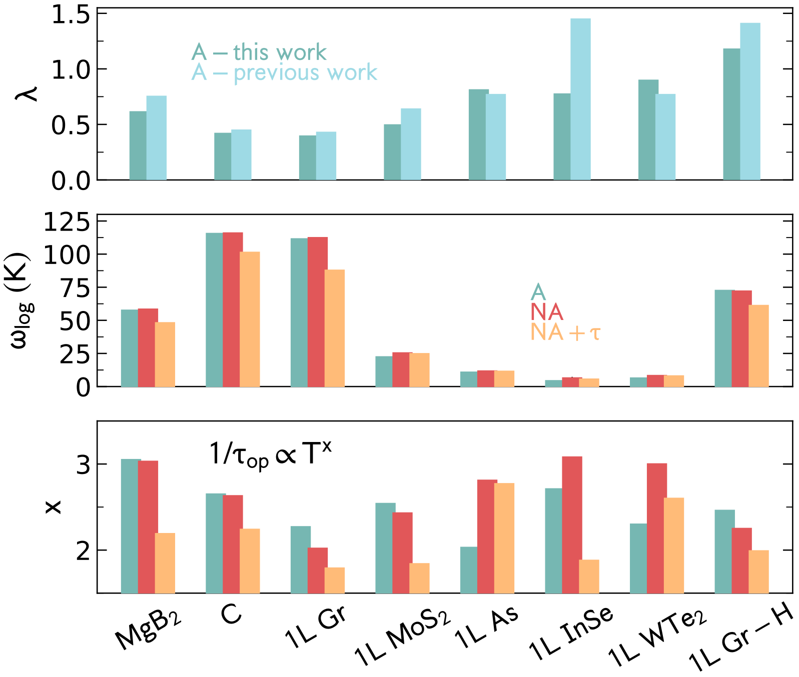


**Supplementary Figure 4**. Upper panel: Comparison between our results for the adiabatic electron-phonon coupling strength $\lambda$, and previously obtained values from the literature. Previous results are from: $MgB_2$ [2], C [3], 1L Gr [4], 1L $MoS_2$ [5], 1L As [6], 1L InSe [7], 1L $WTe_2$ [8], 1L Gr-H [9]. For the doped systems, we have chosen the results from the literature that correspond to the exact same or very similar charge carrier concentration. The difference in calculated adiabatic $\lambda$ for 1L InSe probably comes from different computational details used in Ref. [7]. This difference in calculated $\lambda$ is not entierly surprising considering how sensitive various properties of InSe are on the doping concentration [7, 10]. Middle panel: The values of $\omega_{\rm log}$ that enters Allen-Dynes version of the McMillan's formula as obtained with A, NA, and NA+$\tau$ approaches. The variations of the temperature scaling in optical relaxation rate (i.e., $1/\tau_{\rm op} = B + AT^x$) for small temperatures and frequencies as obtained with A, NA, and NA+$\tau$ approaches.

## Supplementary Note 1. Computational details

The ground state calculation for highly-doped 1L Gr yields a relaxed lattice constant of 2.448 Å with the periodic images separated by 12 Å. High doping regime is achieved by the excess electron charge of 0.67 electrons per unit cell. We use Methfessel-Paxton smearing with 0.01 Ry combined with a 48 × 48 × 1 k-point mesh. For the phonon calculation we use a 24 × 24 × 1 q-point mesh. MLWFs for the EPW calculation are obtained with $sp^2$ and $p_z$ orbitals on the C site along with two $s$ orbitals slightly above/below the midpoint between the two C atoms. For the interpolation, we use a 400 × 400 × 1 and 200 × 200 × 1 fine k- and q-meshes, respectively.

For 1L Gr-H doped with 0.1 h/u.c. the relaxed unit cell is 2.5 Å with the periodic replicas 18 Å apart. Here we use Fermi-Dirac smearing with 0.01 Ry together with a 48 × 48 × 1 k- and 24 × 24 × 1 q-point meshes for the SCF and phonon calculations. MLWFs are obtained from the initial projections of $sp^3$ and $p_z$ orbitals on one C atom. We again use 400 × 400 × 1 and 200 × 200 × 1 fine k- and q- meshes for the EPW calculation.

The self-consistent calculation details for $MoS_2$ include separation of periodic images by 16 Å and the relaxed lattice constant of 3.186 Å. The Fermi level crosses the K valley by 200 meV and just barely touches the Q valley, which is achieved by excess carrier concentration of 0.08 e/u.c. We use Gaussian smearing with 2 mRy together with 48 × 48 × 1 k-point mesh. Phonons are calculated on a 24 × 24 × 1 q-point mesh. For the Fourier interpolation, we use MLWFs with 5 Mo-$d$ orbitals and 3 S-$p$ orbitals on the two S atoms as initial projections. We use a 480 × 480 × 1 and 160 × 160 × 1 fine k- and q-meshes respectively for the interpolation.

The relaxed unit cell constant for 1L As is 3.597 Å with periodic layers separated by 18 Å. We use excess charge of 0.1 e/u.c. For the SCF and phonon calculations we use a 24 × 24 × 1 k-point and 12 × 12 × 1 q-point grids with

Fermi-Dirac smearing of 0.01 Ry. Here we use automatically generated MLWFs using a selected columns of the density matrix (SCDM) approach [11] with parameters $\mu = -6$ and $\sigma = 2.5$ based on the electronic structure of arsenene. The fine k- and q-point meshes are $480 \times 480 \times 1$ and $84 \times 84 \times 1$, respectively.

For 1L InSe, we obtain the relaxed unit cell constant of 3.9 Å with the periodic layers separated by 27 Å. Hole doping is achieved by the excess charge of 0.3 h/u.c. We use the Fermi-Dirac smearing with 0.01 Ry along with a $48 \times 48 \times 1$ k-point and $12 \times 12 \times 1$ q-point meshes. The EPW calculation is performed with MLWFs obtained from the initial projections of 3 Se-$p$ orbitals. The fine k- and q-point meshes are $360 \times 360 \times 1$ and $120 \times 120 \times 1$, respectively.

As for the orthorhombic $WTe_2$, the relaxation yields unit cell constants $a = 3.425$ Å and $b = 6.222$ Å. We use the Fermi-Dirac smearing with 0.01 Ry in combination with a $24 \times 12 \times 1$ k-point mesh. Total negative charge per unit cell used in our calculations is 0.19. The original phonon calculations are done on a $12 \times 6 \times 1$ coarse q-point grid. For the Fourier interpolation, we use MLWFs with 2 W-d orbitals ($d_{x^2-y^2}$ and $d_{xy}$) and Te-$s$ and Te-$p$ orbitals as initial projections. q- and k-point fine meshes are for this system the same and amount to $180 \times 90 \times 1$.

## Supplementary References


[1] S. Baroni, S. de Gironcoli, A. Dal Corso, and P. Giannozzi, Phonons and related crystal properties from density-functional perturbation theory, Rev. Mod. Phys. **73**, 515 (2001).

[2] E. R. Margine and F. Giustino, Anisotropic migdal-eliashberg theory using wannier functions, Phys. Rev. B **87**, 024505 (2013).

[3] L. Boeri, J. Kortus, and O. K. Andersen, Three-dimensional $mgb_2$-type superconductivity in hole-doped diamond, Phys. Rev. Lett. **93**, 237002 (2004).

[4] E. R. Margine and F. Giustino, Two-gap superconductivity in heavily $n$-doped graphene: Ab initio migdal-eliashberg theory, Phys. Rev. B **90**, 014518 (2014).

[5] P. Garcia-Goiricelaya, J. Lafuente-Bartolome, I. G. Gurtubay, and A. Eiguren, Long-living carriers in a strong electron–phonon interacting two-dimensional doped semiconductor, Communications Physics **2**, 81 (2019).

[6] X. Kong, M. Gao, X.-W. Yan, Z.-Y. Lu, and T. Xiang, Superconductivity in electron-doped arsenene, Chinese Physics B **27**, 046301 (2018).

[7] M. Alidoosti, D. N. Esfahani, and R. Asgari, Charge density wave and superconducting phase in monolayer inse, Phys. Rev. B **103**, 035411 (2021).

[8] W. Yang, C.-J. Mo, S.-B. Fu, Y. Yang, F.-W. Zheng, X.-H. Wang, Y.-A. Liu, N. Hao, and P. Zhang, Soft-mode-phonon-mediated unconventional superconductivity in monolayer $1t^{'}-wte_2$, Phys. Rev. Lett. **125**, 237006 (2020).

[9] G. Savini, A. C. Ferrari, and F. Giustino, First-principles prediction of doped graphane as a high-temperature electron-phonon superconductor, Phys. Rev. Lett. **105**, 037002 (2010).

[10] A. V. Lugovskoi, M. I. Katsnelson, and A. N. Rudenko, Strong electron-phonon coupling and its influence on the transport and optical properties of hole-doped single-layer inse, Phys. Rev. Lett. **123**, 176401 (2019).

[11] V. Vitale, G. Pizzi, A. Marrazzo, J. R. Yates, N. Marzari, and A. A. Mostofi, Automated high-throughput wannierisation, npj Computational Materials **6**, 10.1038/s41524-020-0312-y (2020).
